# Supplementary material for: On Exponential Utility and Conditional Value-at-Risk as Risk-Averse Performance Criteria
Source: arXiv:2108.01771 source file (2023-05-05)
Supplement: Supplementary file 1 [file appendix.tex]

\section{Appendix}\label{appendix}

\input{proof_thm1}
